# Supplementary material for: Topological vortex identification for two-dimensional turbulent flows in doubly periodic domains
Source: arXiv:2410.20010 source file (2025-09-15)
Supplement: Supplementary file 1 [file supplemental_material.pdf]

**SUPPLEMENTARY MATERIAL FOR:  
“TOPOLOGICAL VORTEX IDENTIFICATION FOR  
TWO-DIMENSIONAL TURBULENT FLOWS IN DOUBLY  
PERIODIC DOMAINS”**

1. HAMILTONIAN FLOWS ON COMPACT SURFACES WITH BOUNDARY

We consider a two-dimensional compact manifold  $S$  containing physical boundaries. Notice that any incompressible flow on a compact manifold is Hamiltonian if and only if it has zero harmonic part.

**1.1. Local orbit structures for Hamiltonian flows on the flat torus with physical boundaries.**

1.1.1. *Zero-dimensional structures.* Figure 1 shows all non-degenerate zero-dimensional singular orbits. A center is a singular orbit with infinitely many periodic orbits around it as shown in Figure 1(a). Figure 1(b) is a saddle associated with two separatrices. Figure 1(c) is a  $\partial$ -saddle having one separatrix inside the domain and two separatrices along the boundary.

1.1.2. *One-dimensional structures.* Examples of circuits consisting of one boundary, two or more  $\partial$ -saddles, and their self-connected saddle separatrices are a simply essential self-connected saddle connection in Figure 2(a) and a fully essential self-connected saddle connection in Figure 2(b).

When a saddle separatrix connects the same saddle, it is called self-connected. On the other hand, when it connects two different  $\partial$ -saddles on the same boundary, it is called a (self-connected)  $\partial$ -saddle separatrix. Figure 3(a) shows examples of self-connected saddle separatrices. Saddle separatrices connecting different saddles or  $\partial$ -saddles on different boundaries in Figure 3(b) are called non-self-connected saddle separatrices.

**1.2. Topological structure theorem for the Hamiltonian flows on the flat torus with boundary.** Though Lemma 3.2 in the main article holds for a torus without boundary, if the torus contains physical boundaries, it is possible to have at most one fully essential self-connected saddle connection as shown below.

**Lemma 1.1.** For a structurally stable Hamiltonian flow on the torus with physical boundaries, there exists at most one fully essential saddle connection. Furthermore, if a fully essential saddle connection exists, all other saddle connections are inessential.

*Proof.* As shown in Figure 2(b), a fully essential saddle connection can exist. We will show the uniqueness of a fully essential saddle connection if it exists. Suppose that there exists a fully essential saddle connection  $E$ . By Definition 4 in the main article, the complement  $\mathbb{T}^2 - E$  is inessential. Any saddle connection except for  $E$  is

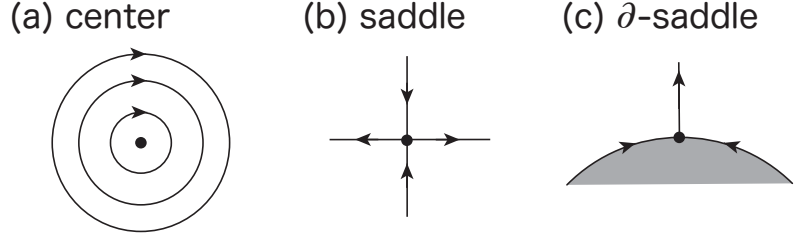

FIGURE 1. Zero-dimensional structures. (a) a center. (b) a saddle. (c) a  $\partial$ -saddle.

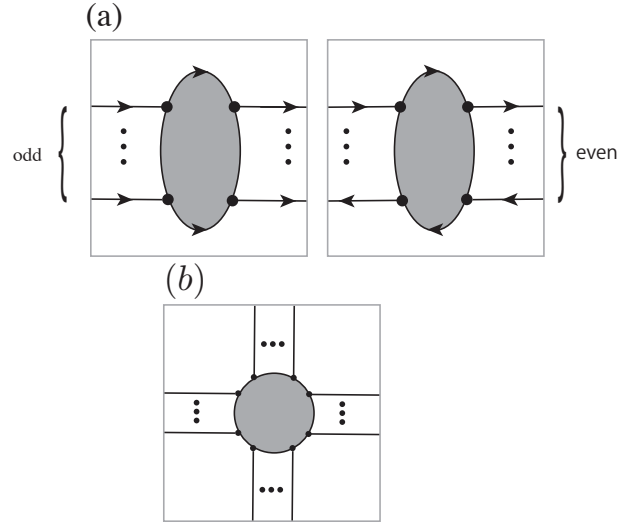

FIGURE 2. One-dimensional structures: Essential saddle connections consisting of one boundary with more than two  $\partial$ -saddles and their self-connected saddle separatrices. (a) Singly essential saddle connections. Note that the orientation of the saddle separatrices varies depending on whether the  $\partial$ -saddle on the boundary is odd or even. (b) Fully essential self-connected saddle connection.

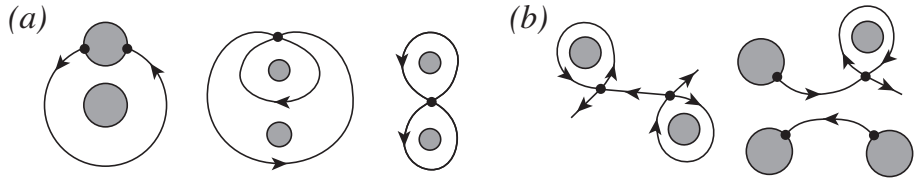

FIGURE 3. Saddle separatrix structures. (a) Self-connected separatrices. (b) Non-self-connected separatrices.

contained in an invariant open disk  $B \subset \mathbb{T}^2 - E$ . This means that the flow contains no essential saddle connections except the fully essential saddle connection  $E$ .  $\square$

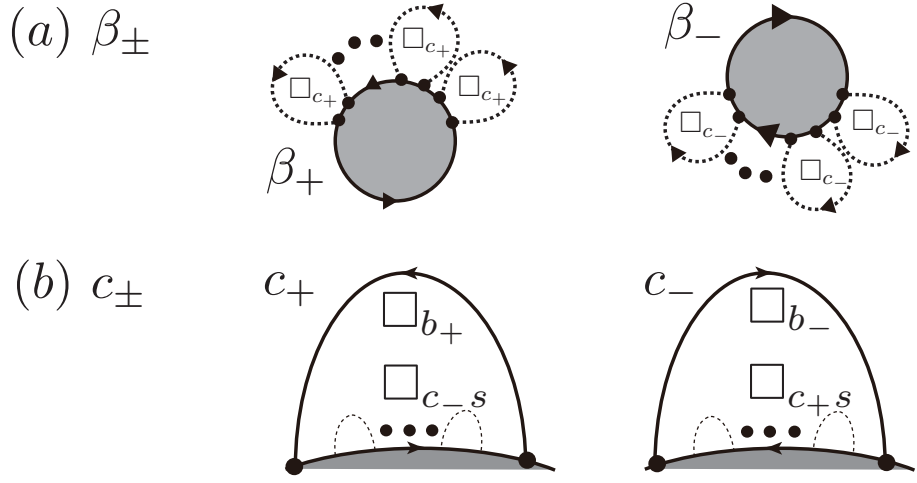

FIGURE 4. One-dimensional structures with inessential self-connected boundary saddle separatrices. (a)  $\beta_{\pm}$  structure: A physical boundary with any number of inessential  $\partial$ -saddle separatrices. When the flow direction along the boundary is counter-clockwise (resp. clockwise), its COT representation is  $\beta_+\{\square_{c_+s}\}$  ( $\beta_-\{\square_{c_-s}\}$ ). (b)  $c_{\pm}$  structures: A one-dimensional structure with any number of  $\partial$ -saddle separatrices filled with periodic orbits inside. The COT symbol is given by  $c_{\pm}(\square_{b_{\pm}}, \square_{c_{\mp}s})$ .

This yields orbit structures of structurally stable Hamiltonian flows on the flat torus with physical boundaries.

**Lemma 1.2.** For a structurally stable Hamiltonian flow on a flat torus with physical boundaries, if the saddle connection diagram contains a singly essential saddle connection, then any other saddle connection is inessential or singly essential.

*Proof.* Let  $C$  be a singly essential saddle connection on a torus. Then,  $\mathbb{T}^2 - C$  consists of an open disk and an essential periodic annulus. Hence, we complete the proof.  $\square$

According to these lemmas, if there exists one singly essential saddle connection then no fully essential saddle connection exists. Conversely, if a fully essential saddle connection exists, then no singly essential saddle connection exists. This is stated in the following dichotomy.

**Corollary 1.3.** One of the following statements holds exclusively for a structurally stable Hamiltonian flow on a flat torus with physical boundaries:

- (1) There exists at most one fully essential saddle connection.
- (2) There exist singly essential saddle connections.

Then the structurally stable Hamiltonian vector field on a flat torus with physical boundaries satisfies the following statement.

**Proposition 1.4.** The following statements hold for a structurally stable Hamiltonian flow on a flat torus with physical boundaries:

- (1) A self-connected saddle connection is either one of the orbit structures in Figure 3 in the main article, Figure 2, and Figure 5(a) as undirected graph up to isotopy on the surface.
- (2) A fully essential saddle connection contains a physical boundary.
- (3) Any singular orbits of the flow are centers, saddles, or  $\partial$ -saddles.

*Proof.* Let  $v$  be the structurally stable Hamiltonian flow on the flat torus  $S$  with physical boundaries. Then any singular orbit of  $v$  is non-degenerate, i.e., saddles,  $\partial$ -saddles, and centers [?, Theorem 3].

We show a fully essential saddle connection contains a physical boundary by contradiction. Suppose that there exists a fully essential saddle connection and that the orbits near all physical boundaries are periodic orbits. Then by collapsing these physical boundaries into single points, we can make it a structurally stable Hamiltonian flow on a flat torus without physical boundaries. However, Lemma 3.2 in the main article implies the non-existence of a fully essential saddle connection, which is a contradiction.

Fix a self-connected saddle connection  $C$ . By Proposition 3.3 in the main article, if  $C$  contains no  $\partial$ -saddles then  $C$  is one of the four kinds of orbit structures in Figure 3 in the main article as an undirected graph up to isotopy on the torus. Suppose that  $C$  contains  $\partial$ -saddles. If  $C$  is inessential, then  $C$  is the orbit structure in Figure 5(a). If  $C$  is singly essential, then  $C$  is the orbit structure in Figure 2(a). If  $C$  is fully essential, then  $C$  is the orbit structure in Figure 2(b).  $\square$

When the torus contains physical boundaries, we have the following equivalent conditions about an essential periodic orbit:

**Lemma 1.5.** The following conditions are equivalent for a periodic orbit  $O$  of a Hamiltonian flow on a torus  $S$  with physical boundaries:

- (1) The periodic orbit  $O$  is essential.
- (2) The periodic orbit  $O$  does not bound a disk in  $S$ , and it is not parallel to a physical boundary.
- (3) The complement  $S - O$  is an annulus with physical boundaries.

*Proof.* A torus  $S$  with physical boundaries can be considered to be contained in the torus  $\mathbb{T}^2$ . Any sufficiently small  $r$ -neighborhood of  $O$  is homotopic to  $O$ . If  $O$  is essential, then  $S - O$  is an annulus with physical boundaries. If  $S - O$  is an annulus with physical boundaries, then  $O$  does not bound a disk in  $S$  and is not parallel to the boundary. If  $O$  does not bound a disk in  $S$  and is not parallel to the boundary, then  $O$  is essential.  $\square$

These lemmas show that by cutting a torus with an essential periodic orbit as shown in Figure 3(b) in the main article, we reduce the Hamiltonian flow on a torus with physical boundaries into one on an annulus. Then, for a Hamiltonian function with a finite number of critical points, we can make its Reeb graph into a tree by cutting one edge corresponding to a domain containing an essential simple closed curve from it. Based on this observation, we assume that the Hamiltonian vector field has an essential periodic orbit in what follows.

**Remark 1.** The existence of essential periodic orbits is not necessarily assured when the torus contains physical boundaries. By Corollary 1.3, a structurally stable Hamiltonian flow has either a fully essential saddle connection or a singly essential

saddle connection exclusively. For the former case, the Hamiltonian flow has no essential periodic orbit, On the other hand, there exists an essential periodic orbit for the latter case. In this paper, we consider a structurally stable Hamiltonian flow on a torus without physical boundaries. Even if a physical boundary exists, the conversion to COT can be defined similarly as long as an essential periodic orbit exists. In Appendix, we will further discuss the conversion to a COT when the torus contains physical boundaries

**1.3. Local orbit structures and COT symbols for Hamiltonian flows on the flat torus with physical boundaries.** Now we list additional orbit structures and their COT symbols for Hamiltonian flow on a torus with physical boundaries, to list all possible structures for structurally stable Hamiltonian flows.

In particular, a fully essential saddle connection with multiple  $\partial$ -saddles in a physical boundary can exist. This is a topologically characteristic feature of flows on the torus when it contains physical boundaries.

## 2. LOCAL ORBIT STRUCTURES OF HAMILTONIAN FLOWS ON A FLAT TORUS WITH PHYSICAL BOUNDARIES AND THEIR COT SYMBOLS

In this paper, aiming at the applications to two-dimensional fluid turbulence in a doubly periodic domain, we have developed the conversion algorithm for Hamiltonian flows on the torus without physical boundaries. However, this is not an essential restriction. We can obtain a similar conversion algorithm to COT and COT representations even if the flow domain contains physical boundaries. In Appendix, we provide the topological classification of local orbit structures in Hamiltonian flows on a torus with physical boundaries and their COT symbols for reference although we won't give the conversion algorithm.

**2.1. Local orbit structures with only inessential saddle connections.** We recall the following structures.

( $\beta_{\pm}$  **structures**) This one-dimensional structure corresponds to a physical boundary with an arbitrary number of  $\partial$ -saddle separatrices as shown in Figure 5(a). When there exist  $\partial$ -saddle separatrices on the boundary and the flow direction along the boundary is counter-clockwise (resp. clockwise), the COT symbol is given as  $\beta_{+}\{\square_{c+s}\}$  (resp.  $\beta_{-}\{\square_{c-s}\}$ ). On the other hand, without any  $\partial$ -saddle separatrix on the boundary, its COT symbol is simply written as  $\beta_{\pm}\{\lambda_{\pm}\}$ . In  $\square_{c\pm s}$ , we arrange the COT symbols for the internal structures in each quasi-essential  $\partial$ -saddle separatrix in a counter-clockwise circular order as follows.

$$\square_{c\pm} = \{c_{+}, c_{-}\}, \quad \square_{c\pm s} := \square_{c\pm} \cdots \square_{c\pm} \quad (s > 0), \quad \square_{c\pm s} := \lambda_{\pm} \quad (s = 0).$$

( $c_{\pm}$  **structures**) There are one-dimensional orbit structures with a boundary attached with a quasi-inessential self-connected  $\partial$ -saddle separatrix as shown in Figure 5(b), whose COT symbols are given by  $c_{\pm}$ . We use the subscript  $+$  (resp.  $-$ ) when the flow direction along the boundary is counter-clockwise (resp. clockwise). In the region enclosed by the  $\partial$ -saddle separatrix and the boundary, a periodic annulus  $\square_{b\pm}$  is necessarily contained, and any number of  $c_{\pm}$  orbit structures can be attached to the boundary. Hence, we can express the orbit structures as  $c_{\pm}(\square_{b\pm}, \square_{c\mp s})$ .

**2.2. Local orbit structures with essential saddle connections.**

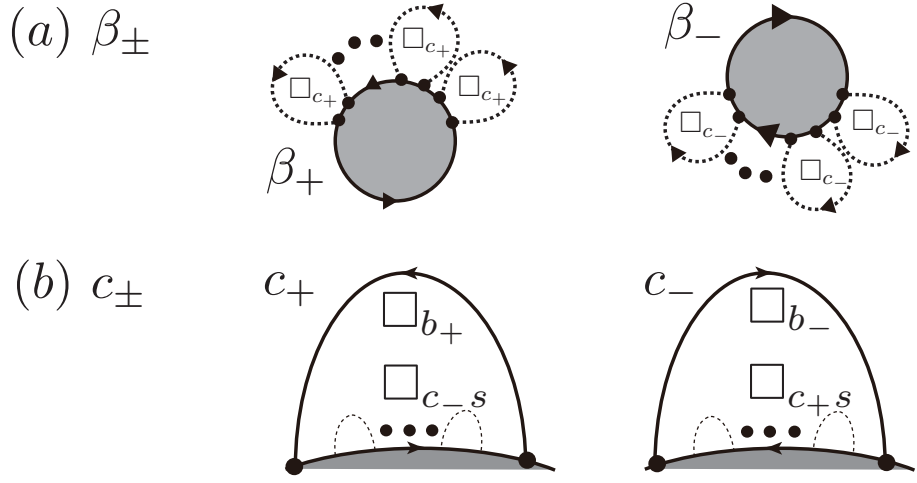

FIGURE 5. One-dimensional structures with inessential self-connected boundary saddle separatrices. (a)  $\beta_{\pm}$  structure: A physical boundary with any number of inessential  $\partial$ -saddle separatrices. When the flow direction along the boundary is counter-clockwise (resp. clockwise), its COT representation is  $\beta_+\{\square_{c+s}\}$  ( $\beta_-\{\square_{c-s}\}$ ). (b)  $c_{\pm}$  structures: A one-dimensional structure with any number of  $\partial$ -saddle separatrices filled with periodic orbits inside. The COT symbol is given by  $c_{\pm}(\square_{b_{\pm}}, \square_{c_{\mp}s})$ .

2.2.1. *Shorthand notations in COT symbols.* According to Lemma 1.1, there are two local orbit structures with essential saddle connections, which are either simply essential or fully essential. When there is a boundary in the flow domain, local orbit structures of structurally Hamiltonian flows can be complex. Some shorthand notations are required to express these structures with COT symbols. For any  $k \in \mathbb{Z}_{>0}$ , we introduce the following shorthand notations.

$$\begin{aligned}
 \square_{C_+} &:= (\square_{b-}, \square_{cs+}, \square_{cs+}) = (\square_{b-}, \square_{cs+}^2), \\
 \square_{C_-} &:= (\square_{b+}, \square_{cs-}, \square_{cs-}) = (\square_{b+}, \square_{cs-}^2), \\
 \square_{C_{+-}} &:= ((\square_{b-}, \square_{cs+}^2), (\square_{b+}, \square_{cs-}^2)) = (\square_{C_+}, \square_{C_-}), \\
 \square_{C_{-+}} &:= ((\square_{b+}, \square_{cs-}^2), (\square_{b-}, \square_{cs+}^2)) = (\square_{C_-}, \square_{C_+}), \\
 (\square_{C_{+-}})^{k+1/2} &:= ((\square_{C_{+-}})^k, \square_{C_+}), \quad (\square_{C_{-+}})^{k+1/2} := ((\square_{C_{-+}})^k, \square_{C_-}), \\
 \square_{\dot{C}_-} &:= (\square_{\dot{+}}, \square_{cs-}), \quad \square_{\dot{C}_+} := (\square_{\dot{-}}, \square_{cs+}).
 \end{aligned}$$

In each  $\square$ , the following can be substituted.

$$\begin{aligned}
 \square_{\dot{+}} &\in \{a_{\pm\dot{+}}, \alpha_{+\dot{-}}, \beta_{2+4k\dot{+}}, \beta_{4+4k\dot{+}}, \lambda_{\dot{+}}\}, \quad \square_{\dot{-}} \in \{a_{\pm\dot{-}}, a_{-\dot{+}}, \beta_{2+4k\dot{-}}, \beta_{4+4k\dot{-}}, \lambda_{\dot{-}}\}, \\
 \square_{b+} &\in \{b_{\pm\dot{+}}, \beta_{\dot{+}}, \beta_{2+4k\dot{+}}, \beta_{4+2(k_1+k_2)+\dot{+}\dot{+}}, \beta_{4+2(k_1+k_2)+\dot{-}\dot{-}}, \beta_{4+2(k+k)+\dot{+}\dot{-}}, \\
 &\quad \beta_{8+2(k_1+k_2)+\dot{+}\dot{+}}, \beta_{4+2(k_1+k_2)+\dot{-}\dot{-}}, \sigma_{\dot{+}}\}, \\
 \square_{b-} &\in \{b_{\pm\dot{-}}, \beta_{\dot{-}}, \beta_{2+4k\dot{-}}, \beta_{4+2(k_1+k_2)-\dot{-}\dot{-}}, \beta_{4+2(k_1+k_2)-\dot{+}\dot{+}}, \beta_{4+2(k+k)-\dot{+}\dot{+}}, \\
 &\quad \beta_{8+2(k_1+k_2)-\dot{-}\dot{-}}, \beta_{4+2(k_1+k_2)-\dot{+}\dot{+}}, \sigma_{\dot{-}}\}.
 \end{aligned}$$

**2.2.2. Orbit structures with singly essential saddle connections.** Let us refer to a separatrix not parallel to the boundary as a *non-boundary-parallel separatrix*. In other words, a non-boundary-parallel separatrix is a separatrix that cannot be continuously transformed in the torus into a separatrix on the boundary while keeping the endpoints on the boundary fixed. The orientation of the separatrices depends on whether the number of non-boundary-parallel separatrices is odd or even. See Figure 6(a). When the number of non-boundary-parallel separatrices on the boundary is odd, the outermost saddle separatrices on the boundary have the same direction. On the other hand, when the number is even, the directions are opposite. The COT symbol of this structure needs to be different depending on the current position and whether the number of non-boundary-parallel separatrices are odd or even. Furthermore, since quasi-essential saddle separatrices can be attached to the boundary, we express their number in the COT symbol.

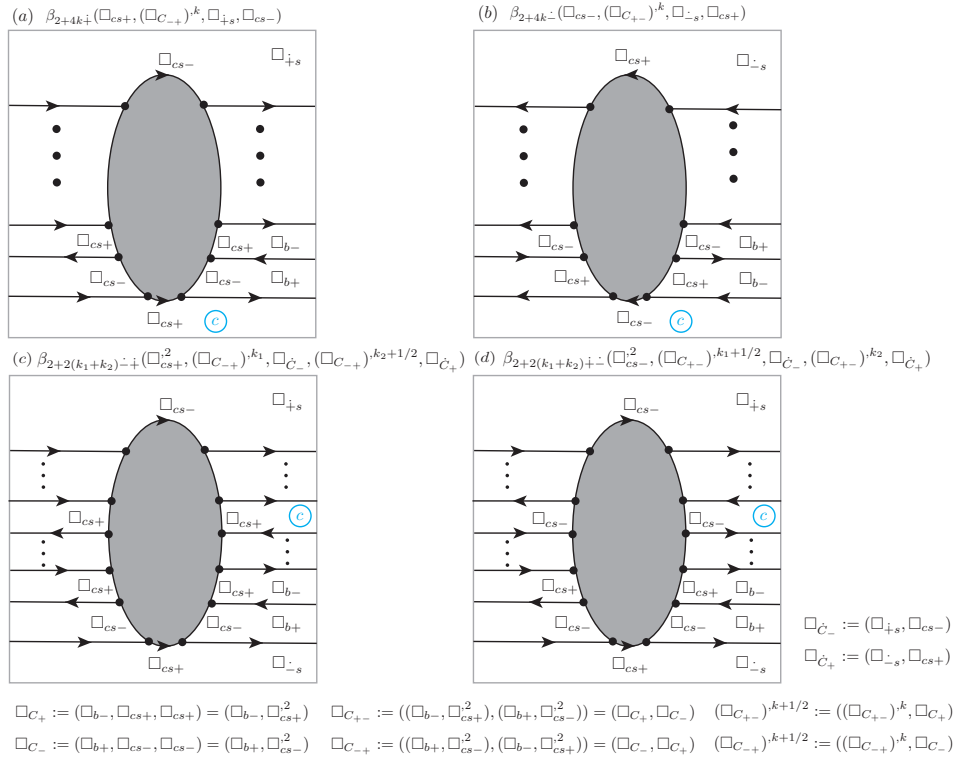

FIGURE 6. List of singly essential saddle connections on the boundary with an odd number of non-boundary-parallel separatrices.

**( $\beta_{2+4k\pm}$ ,  $\beta_{2+2(k_1+k_2)\pm}$  structures)** When there is an odd number of quasi-essential non-boundary-parallel separatrices, four local orbit structures appear as shown in Figure 6. This one-dimensional structure has non-boundary-parallel separatrices connecting the  $1 + 2k$  boundary separatrices and  $4k + 2$   $\partial$ -saddles on the boundary. See Figure 6. Since the saddle connections divide the annular region into  $1 + 2k$  regions, the COT symbol is defined according to the combination of heights

of the Hamiltonian functions in these regions. Accordingly, the orbit structures can be classified into four types as shown in Figure 6.

- Suppose that the current is essential. If the value of the Hamiltonian function in the one-dimensional structure is higher (resp. lower) than that at the current, the COT symbol for this structure is given by  $\beta_{2+4k+}$  (resp.  $\beta_{2+4k-}$ ) as in Figure 6(a) (resp. Figure 6(b)).
- Suppose that the current is inessential. If the value of the Hamiltonian function in the one-dimensional structure is higher (resp. lower) than that at the current, the COT symbol for this structure is given by  $\beta_{2+2(k_1+k_2)+}$  (resp.  $\beta_{2+2(k_1+k_2)-}$ ) as in Figure 6(c) (resp. Figure 6(d)).

Using Figure 6, we specify the COT symbols for the internal orbit structures as follows:

- Figure 6(a)  $\beta_{2+4k+}(\square_{cs+}, (\square_{C-+})^k, \square_{\dot{C}+})$ .
- Figure 6(b)  $\beta_{2+4k-}(\square_{cs-}, (\square_{C+-})^k, \square_{\dot{C}-})$ .
- Figure 6(c)  $\beta_{2+2(k_1+k_2)+}(\square_{cs+}^2, (\square_{C-+})^{k_1}, \square_{\dot{C}-}, (\square_{C-+})^{k_2+1/2}, \square_{\dot{C}+})$ .
- Figure 6(d)  $\beta_{2+2(k_1+k_2)-}(\square_{cs-}^2, (\square_{C+-})^{k_1+1/2}, \square_{\dot{C}-}, (\square_{C+-})^{k_2}, \square_{\dot{C}+})$ .

( $\beta_{4+4k\pm}, \beta_{4+4k\pm}, \beta_{4+2(k_1+k_2)\pm\pm}, \beta_{4+2(k_1+k_2)\mp\pm}$  **structures**) When the number of non-boundary-parallel separatrices of a singly essential saddle connection  $C$  intersecting  $\partial S$  is even, we have the six local orbit structures shown in Figure 7. These one-dimensional structures have non-boundary-parallel separatrices connecting the  $2 + 2k$  boundary separatrices and  $4 + 4k$   $\partial$ -saddles. See Figure 7. Since the annular region is divided into  $2 + 2k$  regions by these saddle connections, the COT symbols must be assigned according to the height of the divided regions. As a result, we obtain the structure shown in Figure 7.

- Suppose that the current is essential. When the value of the Hamiltonian function of the one-dimensional structures is higher (resp. lower) than that at the current, we have the orbit structure of Figure 7(a) (resp. Figure 7(b)) and its COT symbol is given by  $\beta_{4+4k+}$  (resp.  $\beta_{4+4k-}$ ).
- Suppose that the current is inessential. When the value of the Hamiltonian function of the one-dimensional structure is higher than that at the current, and the values of the essential annuli adjacent to saddle connections and the current are equal, we have the orbit structure of Figure 7(c) and its COT symbol is given by  $\beta_{4+2(k_1+k_2)+\pm\pm}$ .
- Suppose that the current is inessential. When the value of the Hamiltonian function of the one-dimensional structure is lower than that at the current, and the values of the essential annuli adjacent to saddle connections and the current are equal, we have the orbit structure of Figure 7(d) and its COT symbol is given by  $\beta_{4+2(k_1+k_2)-\pm\pm}$ .
- Suppose that the current is inessential. When the value of the Hamiltonian function of the one-dimensional structure is lower than that at the current, and the value of the essential annuli adjacent to saddle connections is lower than that at the current, we have the orbit structure of Figure 7(e) and its COT symbol is given by  $\beta_{4+2(k_1+k_2)-\pm\pm}$ .
- Suppose that the current is inessential. When the value of the Hamiltonian function of the one-dimensional structure is higher than that at the current, and the value of the essential annuli adjacent to saddle connections is lower

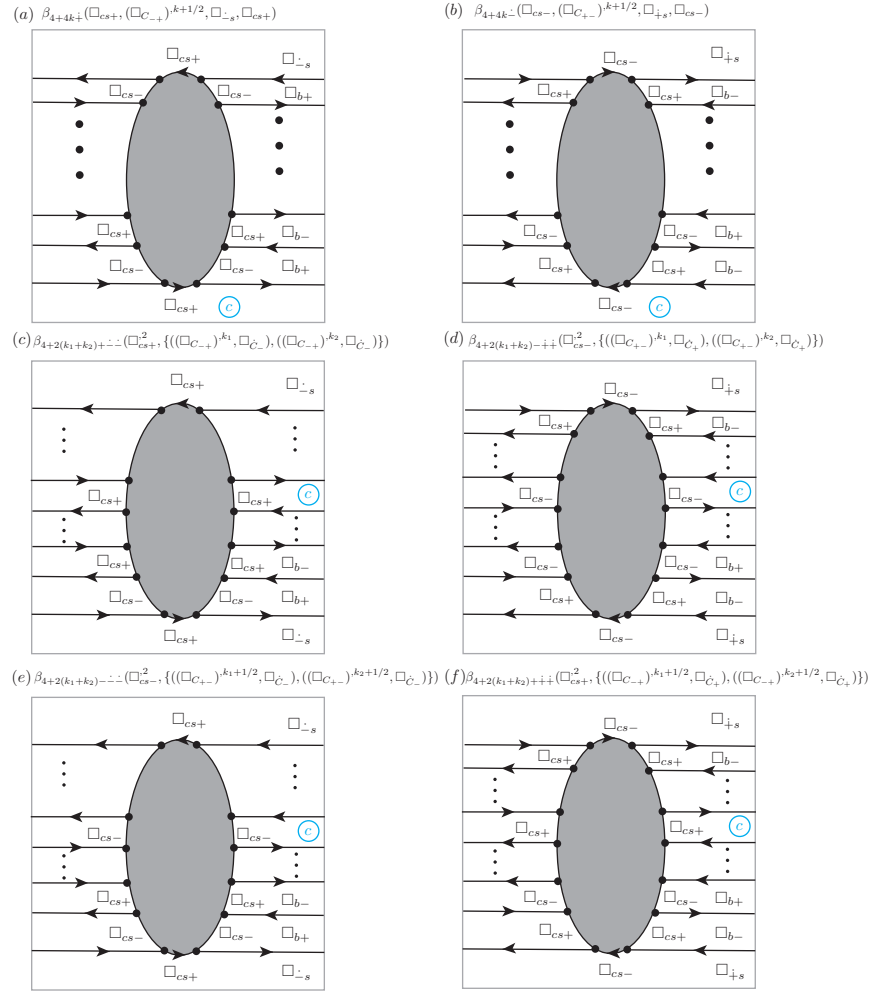

FIGURE 7. List of singly essential saddle connections on the boundary with an even number of non-boundary-parallel separatrices.

than that at the current, we have the orbit structure of Figure 7(f) and its COT symbol is given by  $\beta_{4+2(k_1+k_2)+++}$ .

Using Figure 7, we specify the COT symbols for the internal orbit structures as follows:

- Figure 7(a)  $\beta_{4+4k+}(\square_{cs+}, (\square_{C-+})^{k+1/2}, \square_{\dot{C}+})$ ,
- Figure 7(b)  $\beta_{4+4k-}(\square_{cs-}, (\square_{C+-})^{k+1/2}, \square_{\dot{C}-})$ ,
- Figure 7(c)  $\beta_{4+2(k_1+k_2)+-}(\square_{cs+}^2, \{((\square_{C-+})^{k_1}, \square_{\dot{C}-}), ((\square_{C-+})^{k_2}, \square_{\dot{C}-})\})$ ,
- Figure 7(d)  $\beta_{4+2(k_1+k_2)-++}(\square_{cs-}^2, \{((\square_{C+-})^{k_1}, \square_{\dot{C}+}), ((\square_{C+-})^{k_2}, \square_{\dot{C}+})\})$ ,
- Figure 7(e)  $\beta_{4+2(k_1+k_2)-+-}(\square_{cs-}^2, \{((\square_{C+-})^{k_1+1/2}, \square_{\dot{C}-}), ((\square_{C+-})^{k_2+1/2}, \square_{\dot{C}-})\})$ ,
- Figure 7(f)  $\beta_{4+2(k_1+k_2)+++}(\square_{cs+}^2, \{((\square_{C-+})^{k_1+1/2}, \square_{\dot{C}+}), ((\square_{C-+})^{k_2+1/2}, \square_{\dot{C}+})\})$ ,

in which  $4k = 2k_1 + 2k_2$ . Note that we can choose an essential periodic orbit even if these structures are contained. Hence, we can construct a conversion algorithm for this case in a similar manner.

**2.2.3. Local orbit structures with a fully essential saddle connection.** Lemma 1.1 shows that there exists at most one boundary with fully essential saddle connections. Depending on the location of the current and the flow direction, we need to consider six local orbit structures as shown in Figure 8.

( $\beta_{8+2(k_1+k_2)} \pm$ ,  $\beta_{8+2(k_{1,1}+k_{1,2}+k_2)} \pm \pm$ ,  $\beta_{12+2(k_{1,1}+k_{1,2}+k_2)} \pm \mp$  **structures**) Since the fully essential saddle connection divides the torus  $S$  with boundary into  $8 + 2(k_1 + k_2)$ ,  $8 + 2(k_{1,1} + k_{1,2} + k_2)$ , or  $12 + 2(k_{1,1} + k_{1,2} + k_2)$  regions, it is necessary to assign COT symbols according to the heights of the Hamiltonian functions of the divided regions. As a result, we obtain the following six local orbit structures with different COT symbols as shown in Figure 8.

- Suppose that the current is essential. When the value of the Hamiltonian function of the one-dimensional structure is higher (resp. lower) than that at the current, we have the orbit structure of Figure 8(a) (resp. Figure 8(b)), and its COT symbol is given by  $\beta_{8+2(k_1+k_2)+}$  (resp.  $\beta_{8+2(k_1+k_2)-}$ ).
- Suppose that the current is inessential. When the value of the Hamiltonian function of the one-dimensional structure is lower than that at the current, and the value of the essential annuli adjacent to the saddle connection is lower than that at the current, we have the orbit structure of Figure 8(c), and its COT symbol is given by  $\beta_{8+2(k_{1,1}+k_{1,2}+k_2)}--$ .
- Suppose that the current is inessential. When the value of the Hamiltonian function of the one-dimensional structure is higher than that at the current, and the value of the essential annuli adjacent to the saddle connections is higher than that at the current, we have the orbit structure of Figure 8(d), and its COT symbol is given by  $\beta_{8+2(k_{1,1}+k_{1,2}+k_2)}++$ .
- Suppose that the current is inessential. When the value of the Hamiltonian function of the one-dimensional structure is higher than that at the current, and the value of the essential annuli adjacent to the saddle connections equals that at the current, we have the orbit structure of Figure 8(e), and its COT symbol is given by  $\beta_{12+2(k_{1,1}+k_{1,2}+k_2)}+-$ .
- Suppose that the current is inessential. When the value of the Hamiltonian function of the one-dimensional structure is lower than that at the current, and the value of the essential annuli adjacent to the saddle connections equals that at the current, we have the orbit structure of Figure 8(f), and its COT symbol is given by  $\beta_{12+2(k_{1,1}+k_{1,2}+k_2)}+-$ .

Using Figure 8, we specify the COT symbols for the internal orbit structures as follows:

- Figure 8(a)  $\beta_{8+2(k_1+k_2)+}(\square_{cs+}^4, \{(\square_{C-+})^{k_1+1/2}, (\square_{C-+})^{k_2+1/2}\})$ ,
- Figure 8(b)  $\beta_{8+2(k_1+k_2)-}(\square_{cs-}^4, \{(\square_{C+-})^{k_1+1/2}, (\square_{C+-})^{k_2+1/2}\})$ ,
- Figure 8(c)  $\beta_{8+2(k_{1,1}+k_{1,2}+k_2)}--((\square_{cs-}^2, \{(\square_{C+-})^{k_{1,1}}, (\square_{C+-})^{k_{1,2}}\}, \square_{cs-}^4, \square_{b-}, (\square_{C+-})^{k_2+1/2})$ ,
- Figure 8(d)  $\beta_{8+2(k_{1,1}+k_{1,2}+k_2)}++((\square_{cs+}^2, \{(\square_{C-+})^{k_{1,1}}, (\square_{C-+})^{k_{1,2}}\}, \square_{cs+}^4, \square_{b+}, (\square_{C-+})^{k_2+1/2})$ ,

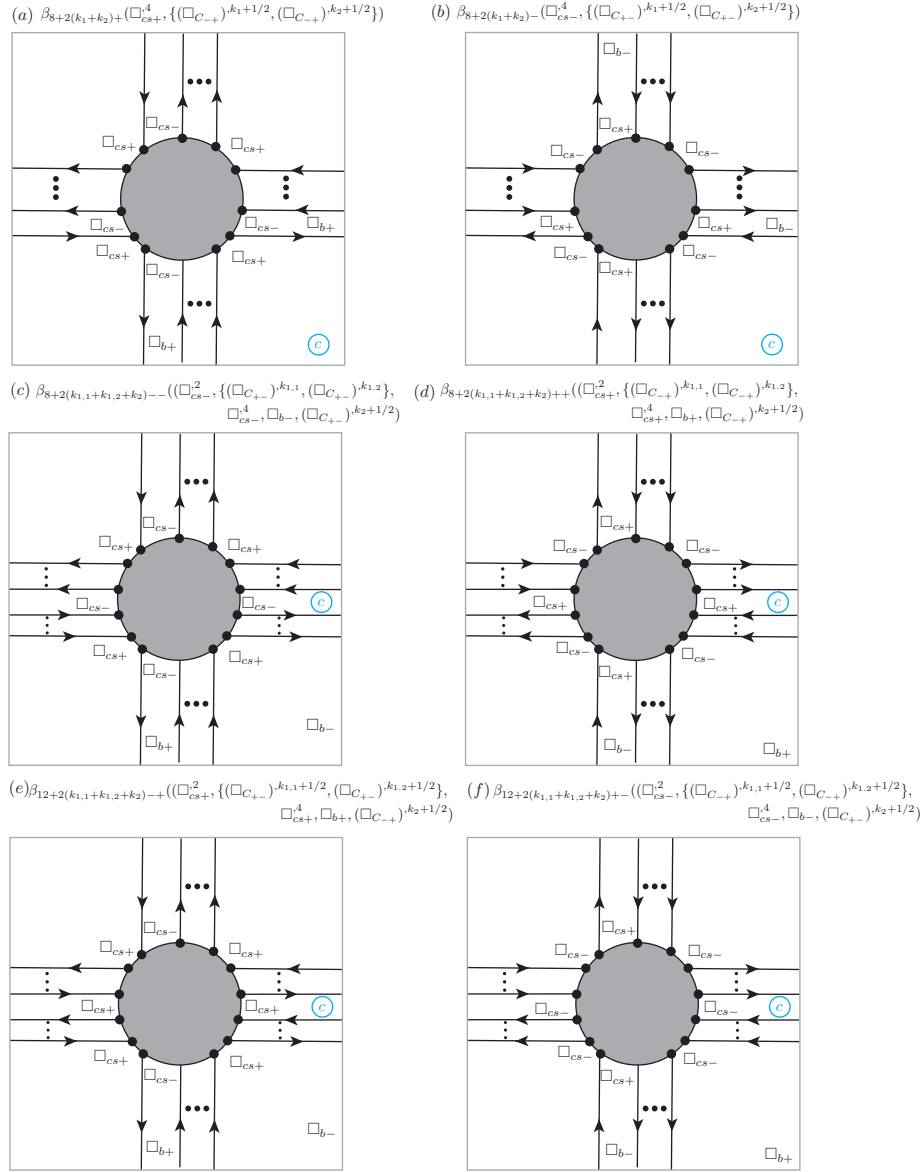

FIGURE 8. List of singly essential saddle connections on the boundary with an even number of non-boundary-parallel separatrices.

- Figure 8(e)  $\beta_{12+2(k_{1,1}+k_{1,2}+k_2)-}((\square_{cs+}^2, \{(\square_{C+-})^{k_{1,1}+1/2}, (\square_{C+-})^{k_{1,2}+1/2}\}), \square_{cs+}^4, \square_{b+}, (\square_{C-+})^{k_2+1/2}),$
- Figure 8(f)  $\beta_{12+2(k_{1,1}+k_{1,2}+k_2)+}((\square_{cs-}^2, \{(\square_{C-+})^{k_{1,1}+1/2}, (\square_{C-+})^{k_{1,2}+1/2}\}), \square_{cs-}^4, \square_{b-}, (\square_{C+-})^{k_2+1/2}),$

where  $k_1, k_2, k_{1,1}, k_{1,2} \geq 0$ . We remark that we have no essential periodic orbit if a fully essential saddle connection exists. Hence, we need to consider a different conversion algorithm in this case.
